# Supplementary material for: Higher-Order Low-Rank Regression
Source: arXiv:1602.06863 source file (2016-02-22)
Supplement: Supplementary file 1 [file supmat.tex]

\begin{theorem}
Let $\mathcal{F}$ be a set of linear tensor functions with Tucker rank penalization, i.e., $\mathcal{F} = \left\{ x\mapsto \W\ttm 1 x : rank(\W) = (R_0,R_1,\ldots,R_p) \right\}$ with $\W\in\mathbb{R}^{d_0\times d_1 \times \ldots \times d_p}$ and $\forall x\in\mathbb{R}^{d_0}$, and let $\mat{x}\in\mathbb{R}^{d_0N}$ with $\|x_n\|^2\leq 1$.
The empirical Rademacher complexity of $\mathcal{F}$ can be upper bounded as follows:
\begin{equation*}
\hat{\mathcal{R}}(\mathcal{F})(\mat{x}) \leq \sqrt{\frac{R_0\times R_1\times\ldots\times R_p}{N}} \sup_{\G}\|\G\|_{max},
\end{equation*}
wehre $\G\in\mathbb{R}^{R_0\times\ldots\times R_p}$ is the core tensor of $\W$.

\end{theorem}

\begin{proof}
\begin{align*}
\hat{\mathcal{R}}(\mathcal{F})(\mat{x}) &= \frac{1}{N} \mathbb{E}_\ten{\sigma} \left[ \sup_{{f}\in\mathcal{F}}  \sum_{n=1}^N \langle \ten{\sigma}^{(n)} , {f}(x_n) \rangle   \right]\\
&=  \frac{1}{N} \mathbb{E}_\ten{\sigma} \left[ \sup_{\W\in\mathbb{R}^{d_0\times  \ldots \times d_p}}  \sum_{n=1}^N \langle \ten{\sigma}^{(n)} , \W\ttm 1x_n \rangle   \right]\\
&=  \frac{1}{N} \mathbb{E}_\ten{\sigma} \left[ \sup_{\W}  \sum_{n=1}^N \langle x_n \otimes \ten{\sigma}^{(n)} , \W \rangle   \right]\\
& \qquad (Cauchy-Schwarz)\\
&\leq  \frac{1}{N}  \sup_{\W} \|\W\| \text{\ }  \mathbb{E}_\ten{\sigma} \left[ \Big\| \sum_{n=1}^N  x_n \otimes \ten{\sigma}^{(n)}\Big\|   \right]\\
& \qquad (Jensen's \ inequality)\\
&\leq  \frac{1}{N}  \sup_{\W} \|\W\| \text{\ }  \left[ \mathbb{E}_\ten{\sigma} \bigg[ \Big\| \sum_{n=1}^N  x_n \otimes \ten{\sigma}^{(n)}\Big\|^2 \bigg]  \right]^{\frac{1}{2}}\\
& \qquad (?)\\
&=  \frac{1}{N}  \sup_{\W} \|\W\| \text{\ }  \Bigg[ \mathbb{E}_\ten{\sigma} \bigg[ \Big\| \mat{X}^{\top} \ten{\sigma}_{(1)}\Big\|^2 \bigg]  \Bigg]^{\frac{1}{2}}\\
&=  \frac{1}{N}  \sup_{\W} \|\W\| \text{\ }  \Bigg[ \mathbb{E}_\ten{\sigma} \bigg[ tr\Big(\ten{\sigma}_{(1)} ^{\top}  \mat{X} \mat{X}^{\top}\ten{\sigma}_{(1)}\Big)  \bigg]  \Bigg]^{\frac{1}{2}}\\
&=  \frac{1}{N}  \sup_{\W} \|\W\| \text{\ }  \Bigg[  tr\bigg(  \mathbb{E}_\ten{\sigma} \Big[\ten{\sigma}_{(1)}\ten{\sigma}_{(1)}^{\top}\Big]  \mat{X} \mat{X}^{\top}\bigg)    \Bigg]^{\frac{1}{2}}\\
&\qquad \big(\mathbb{E}_\ten{\sigma} [\ten{\sigma}_{(1)}\ten{\sigma}_{(1)}^{\top}]   = I\big) \text{\ by the independence and unit-variance of the Rademacher variables}\\
&=  \frac{1}{N}  \sup_{\W} \|\W\| \text{\ }  \bigg[ tr\Big(\mat{X} \mat{X}^{\top}\Big)  \bigg] ^{\frac{1}{2}}\\
& \qquad (\forall 1\leq n\leq N, \|x_n\|^2\leq 1 \Rightarrow tr\Big(\mat{X} \mat{X}^{\top}\Big) \leq N)\\
&\leq  \frac{1}{\sqrt{N}}  \sup_{\W} \|\W\| \text{\ }\\
& \qquad (\| W \| = \| \G \|) \text{\textcolor{blue}{ajouter U orthogonaux et decomposition tucker}}\\
&=  \frac{1}{\sqrt{N}}  \sup_{\G\in\mathbb{R}^{R_0\times\ldots\times R_p}} \|\G\| \text{\ }\\
&\leq \sqrt{\frac{R_0\times R_1\times\ldots\times R_p}{N}} \sup_{\G}\|\G\|_{max}\\
\end{align*}

\textcolor{blue}{verifier notation: $\mat{X}\in\mathbb{R}^{N\times d_0}$ dans la preuve et $\mat{x}\in\mathbb{R}^{d_0 N}$ dans le theorem et definition}

\end{proof}
